# Supplementary material for: From Machine Learning Documentation to Requirements: Bridging Processes with Requirements Languages
Source: arXiv:2511.15340 source file (2025-11-19)
Supplement: Supplementary file 1 [file appendix_more_detailed_criterion.tex]

\begin{longtblr}[
  caption = {Requirements-relevant Info Deductive Codes Criterion (R: Relevant, I: Irrelevant, SRS: software req. specification, SyRS: system req. specification)},
]{
  width = \linewidth,
  colspec = {Q[40]Q[231]Q[365]Q[302]},
  vlines,
  hline{1-2,10,15} = {-}{},
}
Crit. ID & Crit. Description & ISO 29148:2018 References/Rationale & Examples\\
R1 & Explicitly states or clearly implies a need, purpose, goal, or intended use of the model/dataset. & {- 3.1.19 Requirement: "statement which translates or expresses a need and its associated constraints and conditions".\\- 5.2.3 Transformation of needs into requirements: "Defining requirements begins with stakeholder needs (or goals, or objectives)} & DS7:~The dataset was created primarily to serve as training data for ASL to English machine translation.\\
R2 & Describes a specific capability, function, or task the model/dataset performs or supports. & - 5.2.4 Requirements construct: "it shall be met or possessed by a system to solve a problem, achieve an objective..."\textsuperscript{}; "defines the performance of the system... or the corresponding capability of the system..."\textsuperscript{} & MC1:~The model described in this card detects one or more faces in the given image / video.\\
R3 & Specifies performance characteristics or quality attributes, especially if quantitative or verifiable. & {- 5.2.4 Requirements construct: "...it is qualified by measurable conditions..."\textsuperscript{}.\\- 5.2.8.3 Types (Functional/Performance, Quality, Usability)\textsuperscript{}.\\- 9.5.7 Performance requirements (SyRS)\\- 9.6.14 Performance requirements (SRS)\textsuperscript{}} & MC6: InstructGPT outputs are significantly preferred... over outputs from GPT-3 ... produces fewer toxic outputs than GPT-3 on the RealToxicityPrompts dataset, generates more truthful and informative answers on the TruthfulQA dataset...\\
R4 & Defines operational conditions, constraints, or limitations~and negative impacts (e.g., ethical concerns like bias, safety considerations, security vulnerabilities) for the model/dataset's use. & {- 3.1.19 Requirement: "...and its associated constraints (3.1.7) and conditions (3.1.6)"\\- 3.1.7 Constraint: "externally imposed limitation..."\\- 9.6.7 Limitations (SRS)\textsuperscript{},\\- 9.6.16 Design constraints (SRS)\textsuperscript{}\textsuperscript{}} & {MC8:~Although we invested heavily in data cleaning, personally identifiable information may not be entirely eliminated.~\\DS3: ...released the dataset under a Creative Commons Attribution 4.0 International License...}\\
R5 & Describes assumptions or dependencies crucial for the model/dataset's correct or intended functioning. & - 5.2.7 Requirement language criteria: "All assumptions made regarding a requirement shall be documented..." & MC1:~This model needs to be used with NVIDIA Hardware and Software.\\
R6 & Specifies interface details for interaction with the model/dataset. & {- 5.2.8.3 Examples of the requirements type attribute: Interface\textsuperscript{}.\\- 9.5.8 System interface Requirements} & DS1:~Each instance is a frontal or lateral X-ray image...Each image has labels assigned to fourteen observations.\\
R7 & Provides information related to user characteristics or the intended operational environment/context of use. & {- 3.1.8 Context of use\textsuperscript{}.\\- 9.5.4.3 User characteristics (SyRS)\textsuperscript{}.\\- 9.6.6 User characteristics (SRS)\\- 9.4.15 User requirements (StRS)\textsuperscript{}.} & MC7:~RoentGen is intended for research purposes only, with the general purpose of generating chest x-rays based on English radiological text descriptions.\\
R8 & Details evaluation methods, or metrics used, implying how the model/dataset should be assessed or what constitutes acceptable performance. & {- 5.2.5 Verifiable: "...its realization can be proven (verified)... Verifiability is enhanced when the requirement is measurable"\textsuperscript{}.\\- 9.x.18/19 Verification Sec.s (SyRS 9.5.18, SRS 9.6.19)\textsuperscript{}} & MC3:~Our primary evaluation metrics are precision, recall, and F1.\\
I1 & Is purely descriptive of the ML model's architecture or dataset creation process \textit{without} direct implications for its use, performance, capabilities, or constraints. & - 5.2.7 Requirement language criteria: "Requirements should state 'what' is needed, not 'how'"\textsuperscript{}. Unless the "how" imposes a constraint (e.g., a design constraint as per 9.6.16 \textsuperscript{}), it's typically not a requirement itself. & DS7:~A combination of software programs and manual annotations were used to select preexisting YouTube videos.\\
I2 & Provides general ML or domain knowledge not specific to \textit{this} model/dataset's behavior or characteristics. & - 3.1.19 Requirement: "relates to a system, software or service, or other item of interest"\textsuperscript{}. General knowledge is not specific to the item of interest. & DS1:~Chest radiography is the most common imaging examination globally...\\
I3 & Consists of aspirational statements, highly speculative ``future work,'' or desired features not currently implemented or guaranteed. & {- 5.2.5 Necessary: "The requirement is currently applicable and has not been made obsolete by the passage of time"\textsuperscript{}. Future uncommitted work is not ``currently applicable''.\\- 5.2.6 Complete (set): ``The set of requirements... does not contain any To Be Defined (TBD), To Be Specified (TBS), or To Be Resolved (TBR) clauses'' \textsuperscript{} without a plan for resolution. Speculative future work is beyond this.} & {DS8:~In case of updates, we plan to keep the older version of the dataset on the webpage.\\MC10:~We recommend fine-tuning optimizer parameters for the specific dataset at hand...}\\
I4 & Is purely bibliographic, author names, funding acknowledgments, unless imposing a usage constraint. & - The standard's outlines for requirements specifications (Clauses 8, 9) and OpsCon (Annex A) focus on the system's characteristics, needs, and operational context. Bibliographic details are usually in "References" (e.g., 9.2.4 \textsuperscript{}) but are not themselves operational requirements unless they dictate usage. & DS9:~SITUATEDQA was funded by Google Faculty Awards and by UTAustin.\\
I5 & Is raw data within a dataset (e.g., pixel values) as opposed to metadata \textit{about} the dataset or statements regarding its use, quality, or format. & - Requirements are \textit{statements about} the data (e.g., format, quality, constraints on its use), not the data elements themselves. The standard describes requirements \textit{specifications} as structured collections of such statements (e.g., 3.1.27 \textsuperscript{}). & MC9:~The Pororo dataset contains 9 recurring characters, as shown below...
\end{longtblr}
